# Supplementary material for: U-DECN: End-to-End Underwater Object Detection ConvNet with Improved DeNoising Training
Source: arXiv:2408.05780 source file (2025-10-29)
Supplement: Supplementary file 1 [file appendix.tex]

\clearpage
\setcounter{page}{1}
\maketitlesupplementary

% \href{address}{text}
